# Supplementary material for: MetaWeather: Few-Shot Weather-Degraded Image Restoration
Source: arXiv:2308.14334 source file (2024-07-12)
Supplement: Supplementary file 3 [file supp_sidd.tex]

\begin{table*}[t!]
\centering
\caption{Quantitative comparison with VTM~\cite{kim2023universal} on the SIDD~\cite{abdelhamed2018high} dataset. The \textbf{best} results are highlighted.}

\resizebox{0.5\columnwidth}{!}
{
{
\setlength{\tabcolsep}{5pt}
\begin{tabular}{c|cc}
\hline
\toprule
\normalfont{ } 
\multirow{2}{*}{Model} & \multicolumn{2}{c}{SIDD~\cite{abdelhamed2018high}} \\
% \hline
 & PSNR & SSIM \\
\hline
MPRNet~\cite{zamir2021multi} & 17.48 & 0.4720 \\
TransWeather~\cite{valanarasu2022transweather} & 17.34 & 0.4934 \\
NAFNet~\cite{chen2022simple} & 17.67 & 0.4870 \\
WeatherDiffusion~\cite{ozdenizci2023weatherdiffusion} & 6.56 & 0.0050 \\
FocalNet~\cite{cui2023focal} & 17.87 &  0.5007 \\

\textbf{MetaWeather} & 18.63 & 0.4740 \\
\bottomrule
\end{tabular}
}
}

% \vspace{-11pt}
\label{tab:supp_sidd}
\end{table*}
